# Supplementary material for: KARL: Knowledge-Aware Retrieval and Representations aid Retention and Learning in Students
Source: arXiv:2402.12291 source file (2024-10-28)
Supplement: Supplementary file 1 [file online.tex]

\begin{table*}[]
\small
\centering
\setlength{\tabcolsep}{3pt}
\begin{tabular}{@{}cccccc@{}}
\toprule
\textbf{Model} & \textbf{Pre-Test Acc ($\uparrow$)} & \textbf{Post-Test Acc ($\uparrow$)} & \multicolumn{1}{l}{\textbf{Post-Test Recall, C ($\downarrow$)}} & \multicolumn{1}{l}{\textbf{Post-Test Recall, All ($\downarrow$)}} & \multicolumn{1}{l}{\textbf{Post-Test Thruput ($\uparrow$)}} \\ \midrule
KARL & 0.41 & \textbf{0.88} & 6.59 sec & 6.82 sec & 2.581 \\
FSRS & \textbf{0.42} & 0.86 & \textbf{6.16 sec} & \textbf{6.27 sec} & \textbf{2.743} \\ \bottomrule
\end{tabular}
\caption{Comparison of more online evaluation metrics related to medium-term learning measured in our user study. Arrows indicate if higher ($\uparrow$) or lower ($\downarrow$) values are better for each metric. Best results are in \textbf{bold}.}
\label{table:online}
\end{table*}
